# Supplementary material for: Additive relations in irrational powers
Source: arXiv:2512.04081 source file (2026-07-31)
Supplement: Supplementary file 1 [file appendix_rational_case.tex]

%auto-ignore

\section{Rational case}
\label{section/rational_case}

In this section, we consider the equation
\begin{align}
    x_1^c + x_2^c = x_3^c + x_4^c,
    \tag{\ref{additive_energy_equation}}
\end{align}
but with $c$ a rational number, instead of an irrational number, which was already considered in Theorem \ref{irrational_additive_energy_theorem}. In particular, we would like to show that the quantity $B(c, N)$, as defined in (\ref{equation/definition_of_B(c, N)}), is $o(N^2)$. Together with Theorem \ref{irrational_additive_energy_theorem}, this finishes the proof of the sumset corollary stated in the introduction. 

When $c$ is a positive integer, these questions have received plenty of attention over the years. When $c = 2$, the non-trivial solutions overwhelm the trivial ones $B(2, N) \gg N^2(\log{N})^{1/2}$ \cite{Landau_on_the_partition_of_positive_integers_in_four_classes_according_to_the_minimal_number_of_squares_needed_to_their_additive_composition}. Hooley addressed the case $c = 3$ in \cite{Hooley_on_the_representations_of_a_number_as_a_sum_of_two_cubes, Hooley_on_the_numbers_that_are_representable_as_the_sum_of_two_cubes} and arbitrary positive integral $c$ in \cite{Hooley_on_the_representation_of_a_number_as_the_sum_of_two_h-th_powers, Hooley_on_another_sieve_method_and_the_numbers_that_are_a_sum_of_two_h-th_powers}---the third article states the famous conjecture that $B(c, N) = 0$ for integers $c \geq 5$. Greaves \cite{Greaves_on_the_representation_of_a_number_as_a_sum_of_two_fourth_powers} obtained an improvement for $c = 4$ and Skinner--Wooley \cite{Skinner--Wooley_sums_of_two_kth_powers} obtained an improvement for $c \geq 5$ using the Bombieri--Pila determinant method. The further improvements of Heath-Brown \cite{Heath-Brown_the_density_of_rational_points_on_curves_and_surfaces} and Browning \cite{Browning_equal_sums_of_two_kth_powers} for $c \geq 6$ also use the determinant method, together with geometric insights that allow for clever choices of plane sections. Recently, Salberger \cite[Corollary 0.7]{Salberger_counting_rational_points_on_projective_varieties} has shown that
\begin{align}
    \label{equation/positive_integer_estimate_for_nontrivial_solutions}
    B(c, N) \ll_c N^{3/\sqrt{c}}(\log{N})^4 + 1
\end{align}
for $c \geq 2$. When $c = -d$ is a negative integer, the equation (\ref{additive_energy_equation}) is equivalent to the equation
\begin{align}
    \label{equation/additive_energy_for_negative_integer_exponents}
    (x_2 x_3 x_4)^d + (x_1 x_3 x_4)^d = (x_1 x_2 x_4)^d + (x_1 x_2 x_3)^d,
\end{align}
and applying \cite[Theorem 0.5]{Salberger_counting_rational_points_on_projective_varieties} to the projective surface in $\P^3_{\Q}$ of degree $3d$ defined by (\ref{equation/additive_energy_for_negative_integer_exponents}) shows that
\begin{align}
    \label{equation/negative_integer_estimate_for_nontrivial_solutions}
    B(c, N) \ll_d N^{\sqrt{3/\abs{c}}}(\log{N})^4 + N
\end{align}
when $c$ is a negative integer.

The results of the last paragraph can be explained in terms of the Diophantine geometry of the surface $X_c \subseteq \P^3_\Q$ defined by (\ref{additive_energy_equation}). The surface $X_3$ is rational over $\Q$, and so there are many nontrivial rational points. In particular, they are Zariski dense in $X_3$. The surface $X_4$ is K3 and admits an elliptic fibration with generic fibre having Mordell--Weil rank one. The rational points of $X_4$ are again Zariski dense (even dense in the real topology) \cite{Swinnerton-Dyer_A4+B4=C4+D4_revisted}. Finally, the surfaces $X_c$ for $c \geq 5$ are of general type, and the conjecture that $X_c$ contains no nontrivial rational points can be regarded as a manifestation of the Bombieri--Lang conjecture, wherein the rational points of $X_c$ are not Zariski dense, in contrast to the cases $c \in \{3, 4\}$.

Let $c = a/q$ be an arbitrary rational number not in $\{0, 1, 2\}$. The strategy to estimate $B(a/q, N)$ in this case employs a result of Carr--O'Sullivan \cite[Theorem 1.1]{Carr--O'Sullivan_on_the_linear_independence_of_roots} about linear independence of $a/q$-powers to reduce to the problem of estimating $B(a, M)$ for various $M \leq N^{1/q}$. This is the content of Proposition \ref{proposition/reduction_of_rational_additive_energy_to_integer_case}. The problem of estimating $B(a, M)$ can be handled using, for example, Salberger's results \cite[Theorem 0.5, Corollary 0.7]{Salberger_counting_rational_points_on_projective_varieties}, which we have mentioned already. This results in the following estimates for $B(a/q, N)$. In fact, for $c \in \{1/2, 1/3\}$ we obtain asymptotic formulae.

\begin{theorem}
    \label{theorem/additive_energy_in_the_rational_case}
    Let $N \geq 2$ be an irrational number.
    \begin{enumerate}[(1)]
        \item We have the asymptotic formulae
        \begin{align*}
            B(1/2, N) &= \zeta(3/2)N^{3/2} + O(N\log{N}), \\
            B(1/3, N) &= N(\log{N}) + O(N).
        \end{align*}
        \item For $q > 3$ we have $B(1/q, N) \ll N$, and for $q > 2$ we have
        \begin{align*}
            B(2/q, N) \ll \frac{N(\log{N})^3}{q^2}.
        \end{align*}
        \item For a rational number $a/q$ in lowest terms, and with $a < 0$ or $a > 2$, we have
        \begin{align*}
            B(a/q, N) \ll_a \frac{N(\log{N})^4}{q^3}.
        \end{align*}
    \end{enumerate}
\end{theorem}

We now prove some auxiliary results that are required to establish Theorem \ref{theorem/additive_energy_in_the_rational_case}.

\begin{proposition}
\label{proposition/reduction_of_rational_additive_energy_to_integer_case}
    Let $a$ and $q > 0$ be coprime integers, and let $\vec{x} = (x_1, x_2, x_3, x_4)$ be a non-trivial solution to (\ref{additive_energy_equation}) with $c = a/q$. Then we can write $x_i = a_i^q b$ for $i \in \{1, 2, 3, 4\}$, where $\vec{a} = (a_1, a_2, a_3, a_4)$ is a non-trivial solution to (\ref{additive_energy_equation}) with $c = a$, and $b$ is a positive integer. In particular, for $N$ a positive integer we have
    \begin{align*}
        B(a/q, N) = \sum_{b \leq N} B(a, (N/b)^{1/q}).
     \end{align*}
\end{proposition}
\begin{proof}
    Suppose $\vec{x}$ is a non-trivial solution to (\ref{additive_energy_equation}) and let $x_i = a_i^qb_i$ where $a_i, b_i \in [N]$ and the $b_i$ are $q$-th power free. Consider the set $A = \{b_1^{a/q}, b_2^{a/q}, b_3^{a/q}, b_4^{a/q}\}$ inside $L = \Q(b_1^{1/q}, b_2^{1/q}, b_3^{1/q}, b_4^{1/q})$. If $z, w \in \{b_1, \dots, b_4\}$ and $z^{a/q}$ and $w^{a/q}$ are $\Q$-linearly dependent, then let $s$ and $t$ be coprime integers with $sz^{a/q} = tw^{a/q}$. If $p$ is a prime dividing $s$, then
    \begin{align*}
        qv_p(s) + av_p(z) = av_p(w)
    \end{align*}
    so that $a \mid v_p(s)$. Therefore $s = u^a$ for some integer $u$, and similarly $t = v^a$. We now have
    \begin{align*}
        z = \bigg(\frac{v}{u}\bigg)^qw,
    \end{align*}
    so $z = w$, since $z$ and $w$ are $q$-th power free. In the notation of \cite{Carr--O'Sullivan_on_the_linear_independence_of_roots}, this means that $A \in \theta(\Q, L)$, and so $A$ is $\Q$-linearly independent by Theorem 1.1 in \textit{loc. cit.}. Substituting the expressions for the $x_i$ into (\ref{additive_energy_equation}) yields
    \begin{align*}
        a_1^ab_1^{a/q} + a_2^ab_2^{a/q} = 
        a_3^ab_3^{a/q} + a_4^ab_4^{a/q}.
    \end{align*}
    Since the $a_i$ are nonzero, we know that $b_1$ must be equal to at least one of $b_2, b_3$ or $b_4$. If it is equal to $b_2$, but not $b_3$ or $b_4$, then $a_1 = a_2 = 0$, and so $b_1$ must be equal to at least one of $b_3$ and $b_4$. If it is only equal to say $b_3$, then $a_1 = a_3$, so $a_2 = a_4$ and we have a trivial solution. Therefore $b_1 = b_2 = b_3 = b_4$. In particular, every nontrivial solution takes the form
    \begin{align*}
        x_i = a_i^qb
    \end{align*}
    for some $a_i \in [N^{1/q}]$ and $b \in [N]$, such that $\vec{a}$ is a nontrivial solution to
    \begin{align*}
        a_1^a + a_2^a = a_3^a + a_4^a.
    \end{align*}
    It follows that
    \begin{align*}
        B(a/q, N) &= \sum_{b \leq N} B(a, (N/b)^{1/q}).
    \end{align*}
\end{proof}

The following lemma can be proved using partial summation \cite[Theorem 3.2]{Apostol_introduction_to_analytic_number_theory}, but we state it here for convenience.

\begin{lemma}
\label{summation_lemma}
    Let $\alpha > 0$ and let $N$ be a positive integer. Then
    \begin{align*}
        \sum_{b \leq N} \bigg(\frac{N}{b}\bigg)^{\alpha} =
        \begin{cases}
            N(\log{N}) + O(N) & \alpha = 1, \\
            \frac{N}{1 - \alpha} + \zeta(\alpha)N^{\alpha} + O(1) & \alpha \neq 1,
        \end{cases}
    \end{align*}
    where the big-$O$ constant does not depend on $\alpha$.
\end{lemma}

The following upper bound for $B(2, N)$ will be useful in the proof of Theorem \ref{theorem/additive_energy_in_the_rational_case}.

\begin{lemma}
\label{upper_bound_for_additive_energy_of_squares}
    For $N \geq 2$ we have $B(2, N) \ll N^2(\log{N})^3$.
\end{lemma}
\begin{proof}
    We thank Akshat Mudgal for showing us this argument. For $n \leq 2N^2$ let
    \begin{align*}
        r(n) = \card\{(x, y) \in [N]^2 : n = x^2 - y^2\}.
    \end{align*}
    If $n = x^2 - y^2$ then $x - y$ divides $n$. If $d = x - y$ then we can recover $x$, and therefore $y$, from $d$ because of the relation $2x = d + n/d$. Thus $r(n) \leq \sigma_0(n)$, where $\sigma_0$ is the divisor counting function. Then
    \begin{align*}
        B(2, N) \leq 
        \sum_{n \leq 2N^2} r(n)^2
        \leq
        \sum_{n \leq 2N^2} \sigma_0(n)^2
        \ll N^2(\log{N})^3,
    \end{align*}
    where the second moment estimate for the divisor function can be found in \cite{Luca--Toth_the_r-th_moment_of_the_divisor_function}.
\end{proof}

\noindent\textbf{Proof of Theorem \ref{theorem/additive_energy_in_the_rational_case}.}
Suppose first that $a = 1$. Then Proposition \ref{proposition/reduction_of_rational_additive_energy_to_integer_case} yields
\begin{align*}
    B(1/q, N) &= \sum_{b \leq N} \floor{\bigg(\frac{N}{b}\bigg)^{1/q}}^3
    \\ &=
    \sum_{b \leq N}
    \bigg(
    \bigg(\frac{N}{b}\bigg)^{1/q}
    + O(1)
    \bigg)^3
    \\ &=
    \sum_{b \leq N} \bigg(\frac{N}{b}\bigg)^{3/q} +
    O\bigg(
    \sum_{b \leq N} \bigg(\frac{N}{b}\bigg)^{2/q} 
    \bigg),
\end{align*}
and two applications of Lemma \ref{summation_lemma} give
\begin{align*}
    B(1/2, N) &= \zeta(3/2)N^{3/2} + O(N\log{N})
    \quad\quad (q = 2), \\
    B(1/3, N) &= N\log{N} + O(N) \quad\quad (q = 3), \\
    B(1/q, N) &\ll qN \quad\quad (q > 3).
\end{align*}
When $a = 2$, we use the upper bound in Lemma \ref{upper_bound_for_additive_energy_of_squares} to obtain
\begin{align*}
    B(2/q, N) &\ll
    \frac{(\log{N})^3}{q^3}
    \sum_{b \leq N} \bigg(\frac{N}{b}\bigg)^{2/q}
    \\ &\ll
    \frac{(\log{N})^3}{q^3}
    \bigg(
    \frac{N}{1 - 2/q} + \zeta(2/q)N^{2/q} + 1 
    \bigg)
    \\ &\ll \frac{N(\log{N})^3}{q^2}.
\end{align*}
When $a > 2$, we use \cite[Corollary 0.7]{Salberger_counting_rational_points_on_projective_varieties} to obtain
\begin{align*}
    B(a/q, N) &\ll_a \frac{(\log{N})^4}{q^4}\sum_{b \leq N}
    \bigg(
    \frac{N}{b}
    \bigg)^{3a^{-1/2}q^{-1}}
    \\ &\ll_a
    \frac{(\log{N})^4}{q^4}
    \bigg(
    \frac{N}{1 - 3a^{-1/2}q^{-1}} +
    \zeta(3a^{-1/2}q^{-1})N^{3a^{-1/2}q^{-1}}
    + 1
    \bigg)
    \\ &\ll_a
    \frac{N(\log{N})^4}{q^3}.
\end{align*}
When $a = -d$ is negative, 
\begin{align*}
    B(a/q, N) &\ll_a \sum_{b \leq N} B(-d, (N/b)^{1/q}) \\
    &\ll_a
    \frac{(\log{N})^4}{q^4}
    \sum_{b \leq N} \bigg(\frac{N}{b}\bigg)^{\sqrt{3}a^{-1/2}q^{-1}} \\
    &\ll_a
    \frac{(\log{N})^4}{q^4}
    \frac{N}{1 - \sqrt{3}q^{-1}} \\
    &\ll_a \frac{N(\log{N})^4}{q^3}.
\end{align*}
This concludes the proof of Theorem \ref{theorem/additive_energy_in_the_rational_case}.

\noindent\textbf{Q.E.D.}
